# Supplementary material for: A First Principles Investigation of Native Interstitial Diffusion in Cr2O3
Source: arXiv:1805.03775 ancillary file (2018-05-11)
Supplement: Supplementary file 1 [file si-interstitial-diff.pdf]

# Supplementary Information to A First Principles Investigation of Native Interstitial Diffusion in $\text{Cr}_2\text{O}_3$

Bharat Medasani,<sup>\*,†</sup> Maria L. Sushko,<sup>†</sup> Kevin M. Rosso,<sup>†</sup> Daniel K. Schreiber,<sup>‡</sup>  
and Stephen M. Bruemmer<sup>‡</sup>

<sup>†</sup>*Physical and Computational Sciences Directorate*

<sup>‡</sup>*Energy and Environment Directorate, Pacific Northwest National Laboratory, Richland,  
WA 99354, USA*

E-mail: bharat.medasani@pnnl.gov,mbkumar@gmail.com

## Density Functional Calculations

We performed the density functional theory (DFT) calculations using the Vienna *ab initio* simulation package (VASP).<sup>1-3</sup> PBEsol<sup>4</sup> generalized-gradient approximation (GGA) for the exchange-correlation functional was used in conjunction with projector augmented wave (PAW) potentials<sup>5,6</sup> optimized for PBE functional. We utilized Hubbard on-site correction with  $U_{eff} = U - J = 3.7$  eV to treat the Cr 3d electrons within the rotationally invariant DFT+U approach by Dudarev et al.<sup>7</sup> A cut-off value of 400 eV was used for the plane-wave basis set based on the convergence for bulk  $\text{Cr}_2\text{O}_3$ . Spin polarization with anti-ferromagnetic (AFM) ordering of Cr spins was used. Gaussian method with a width of 0.02 eV was used for electronic smearing. Based on the convergence tests of defect energies with the supercell size, the  $2 \times 2 \times 1$  supercells (108 atoms) were optimized with  $2 \times 2 \times 2$  Monkhorst-Pack

$k$ -point grid. The atomic positions in the defect supercells were relaxed at constant volume and fixed cell shape until the individual forces on each atom were minimized to 0.01 eV/Å.

## Uncorrected Formation Energies

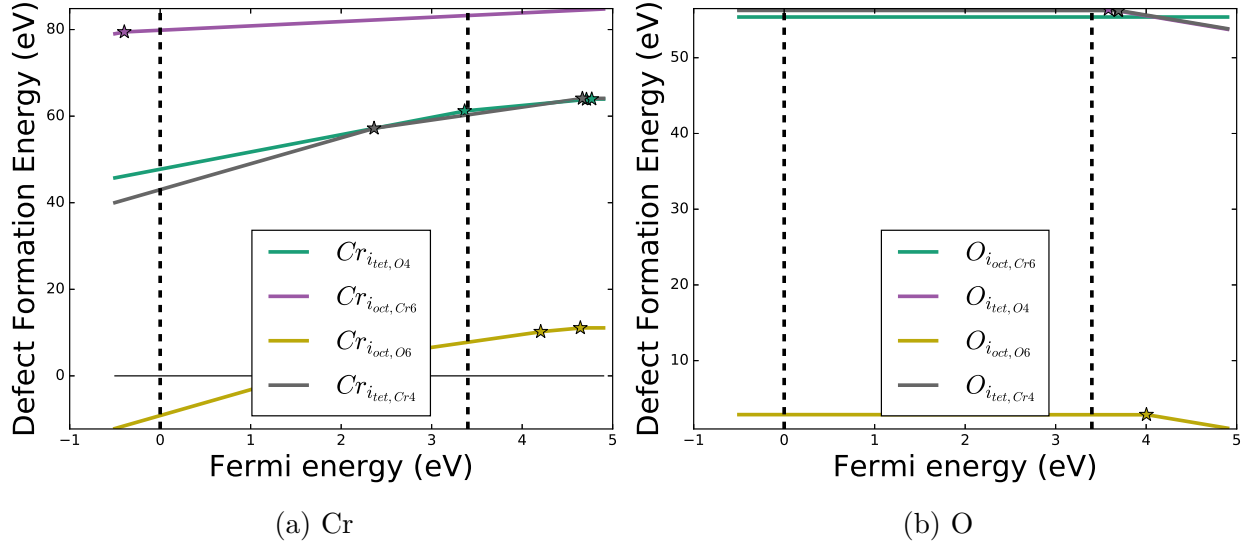

Figure S1: Preliminary formation energies of Cr and O interstitials at the sites shown in Figure 1 in the article with no corrections. Both the plots correspond to O rich conditions.

## Local relaxation surrounding interstitials

Table S1: Relaxation of the atoms surrounding Cr interstitial.

| Atom<br>(q=) | Distance (in Å) | Multiplicity* |   |   |   | Relaxation (in Å) |             |             |               |
|--------------|-----------------|---------------|---|---|---|-------------------|-------------|-------------|---------------|
|              |                 | 0             | 1 | 2 | 3 | 0                 | 1           | 2           | 3             |
| Cr           | 2.1             | 2             | 2 | 2 | 2 | 0.30              | 0.25 – 0.26 | 0.25 – 0.27 | 0.28 – 0.3    |
| Cr           | 2.8             | –             | 2 | 2 | 2 | –                 | 0.11 – 0.13 | 0.1         | 0.11          |
| Cr           | 3.7             | –             | 1 | 1 | – | –                 | 0.11        | 0.11        | –             |
| Cr           | 4.7             | 2             | 1 | 2 | 2 | 0.11              | 0.16        | 0.11 – 0.17 | 0.13 – 0.19   |
| O            | 2.1             | 1             | 1 | 1 | 2 | 0.11              | 0.15        | 0.14        | -0.12 – -0.15 |
| O            | 3.7             | 2             | 5 | 2 | 3 | 0.11              | 0.11 – 0.22 | 0.12        | 0.11          |
| O            | 4.6             | –             | 1 | – | – | –                 | 0.11        | –           | –             |

\* Indicates number of sites with displacements  $> 0.1$  Å.

Table S2: Relaxation of the atoms surrounding O interstitial. Only displacements  $> 0.1\text{\AA}$  are listed.

| Atom<br>(# of atoms) | Unrelaxed<br>Distance ( $\text{\AA}$ ) | Relaxation ( $\text{\AA}$ ) |             |      |
|----------------------|----------------------------------------|-----------------------------|-------------|------|
|                      |                                        | q=0                         | q=-1        | q=-2 |
| Cr(2)                | 1.9                                    | 0.12 – 0.13                 | –           | –    |
| O(2)                 | 2.7                                    | –                           | 0.13 – 0.15 | 0.36 |
| O(2)                 | 2.9                                    | –                           | 0.16 – 0.18 | 0.23 |

## Influence of $U_{O_{2p}}$ on hole localization

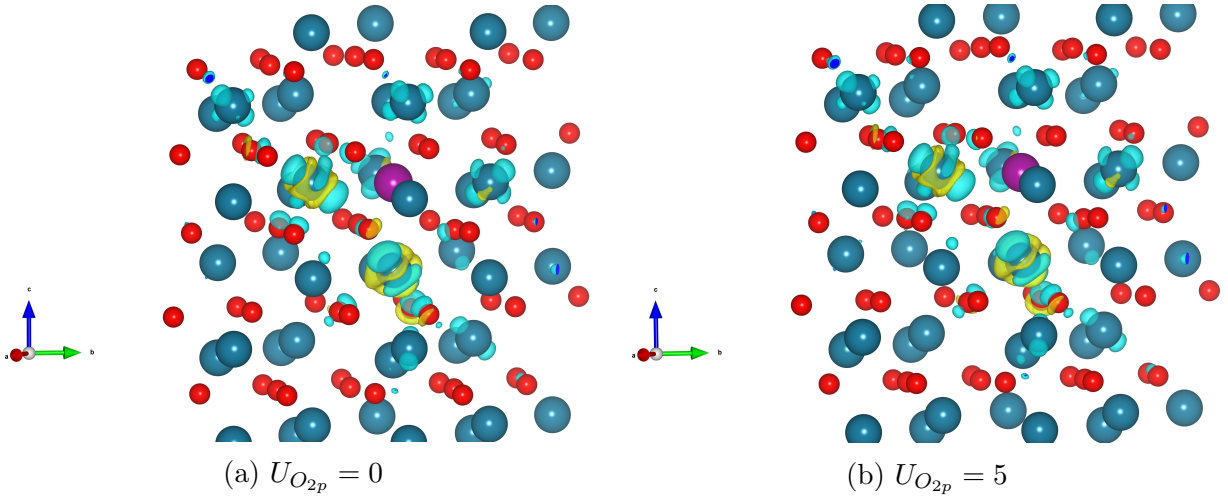

Figure S2: Distribution of  $Cr_i^1$  hole charge with  $U_{O_{2p}}$  values of 0 and 5.

## Corrections to *Ab Initio* Interstitial Formation Energies

### Anisotropic Electrostatic Correction

The interstitial formation energies were first corrected for spurious electrostatic interactions due to the periodic boundary conditions and the interaction of the defect with the compensating background charge. Electrostatic corrections are obtained with anisotropic FNV (Freysoldt, Neugebauer, and Vande Walle) method developed by Kumagai and Oba.<sup>8,9</sup> Table S3 lists the electrostatic corrections. The data show that the magnitude of finite size electrostatic error is significant for charged interstitials and the magnitude of correction

increases with interstitial charge.

Table S3: Electrostatic corrections to the interstitial formation energies of  $\text{Cr}_2\text{O}_3$  obtained with PyCDT<sup>10</sup> using extended Freysoldt method.<sup>8,9</sup>

| Defect | q  | Correction (eV) |       |
|--------|----|-----------------|-------|
|        |    | GGA             | GGA+U |
| $O_i$  | 0  | 0.000           | 0.000 |
|        | -1 | 0.556           | 0.088 |
|        | -2 | 1.200           | 0.435 |
| $Cr_i$ | 0  | 0.000           | 0.000 |
|        | 1  | 0.205           | 0.334 |
|        | 2  | 0.532           | 0.802 |
|        | 3  | 0.941           | 1.598 |

## Bandgap Related Corrections

After accounting for the electrostatic corrections, the transition levels of the Cr and O interstitials with respect to the valence band maximum were corrected for the DFT bandgap error with the scheme proposed by Janotti and Vande Walle. The transition level data in Table S4 shows that GGA+U predicted  $Cr_i$  and  $O_i$  transition levels are in the upper region of the bandgap and higher than the GGA predicted levels. The computed corrections to GGA+U transition levels from the GGA and GGA+U transition levels shift the transition levels downwards.

The resulting corrections to the interstitial formation energies given in Table S6 indicate that the bandgap correction scheme reduces the formation energies of the interstitials. This is in contrast to that of the vacancies, where except for  $V_O^0$ , the formation energies increased due to bandgap error correction. The magnitude of correction to interstitial formation energies increases with the occupancy of the defect energy levels by electrons. Here,  $O_i^0$  has an occupancy of 0 and  $O_i^{-2}$  has 2. For Cr interstitials, the occupancy is inversely proportional to the magnitude of defect charge. The correction significantly reduces the formation energies of all electron occupied interstitials except  $O_i^{-1}$ , where a relatively small reduction of -0.23 eV is observed.

Table S4: Uncorrected and corrected defect transition levels for chromium and oxygen interstitials. The defect transition levels are computed after applying electrostatic corrections, which are given in Tab. S3. The corrections shown in 5th column are computed using the scheme proposed in Ref. 11.

| Defect | $q/q'$ | $\epsilon^{\text{GGA}}(q/q')$ | $\epsilon^{\text{GGA+U}}(q/q')$ | $\epsilon_{\text{corr}}(q/q')$ | $\epsilon(q/q')$ |
|--------|--------|-------------------------------|---------------------------------|--------------------------------|------------------|
| $O_i$  | -1/0   | 0.22                          | 2.53                            | 0.68                           | 3.21             |
|        | -2/0   | 0.82                          | 2.35                            | 0.45                           | 2.8              |
|        | -2/-1  | 1.42                          | 2.17                            | 0.22                           | 2.39             |
| $Cr_i$ | 2/3    | 0.93                          | 1.48                            | 0.16                           | 1.64             |
|        | 1/3    | 1.10                          | 1.89                            | 0.23                           | 2.13             |
|        | 1/2    | 1.26                          | 2.30                            | 0.31                           | 2.61             |
|        | 0/3    | 1.12                          | 2.12                            | 0.30                           | 2.42             |
|        | 0/2    | 1.20                          | 2.45                            | 0.36                           | 2.81             |
|        | 0/1    | 1.15                          | 2.59                            | 0.42                           | 3.02             |

Table S5: Bandgap correction to the interstitial formation energies of  $\text{Cr}_2\text{O}_3$ . The corrections are computed using the scheme proposed in Ref. 11.

| Defect | q  | Occupancy | Correction |
|--------|----|-----------|------------|
| $O_i$  | 0  | 0         | 0          |
|        | -1 | 1         | 0.68       |
|        | -2 | 2         | 0.90       |
| $Cr_i$ | 0  | 3         | 0.89       |
|        | 1  | 2         | 0.47       |
|        | 2  | 1         | 0.16       |
|        | 3  | 0         | 0.0        |

## Phonon Density of States

To interstitial structures and the transition state structures are validated with phonon density of states (PDOS). The PDOS of transition states and the interstitials were computed using Phonopy.<sup>12</sup> Before computing the phonon spectra, the structures of the transition states and the interstitials were further optimized with a force-based quasi-Newton algorithm until the forces were minimized to 0.001 eV/Å. Based on finite displacement method, 726 displacement cells were generated by Phonopy. The total energy of each of the generated cells was converged to 1e-7 eV, and force constants and dynamical matrix were evaluated from the forces obtained from the converged calculations.

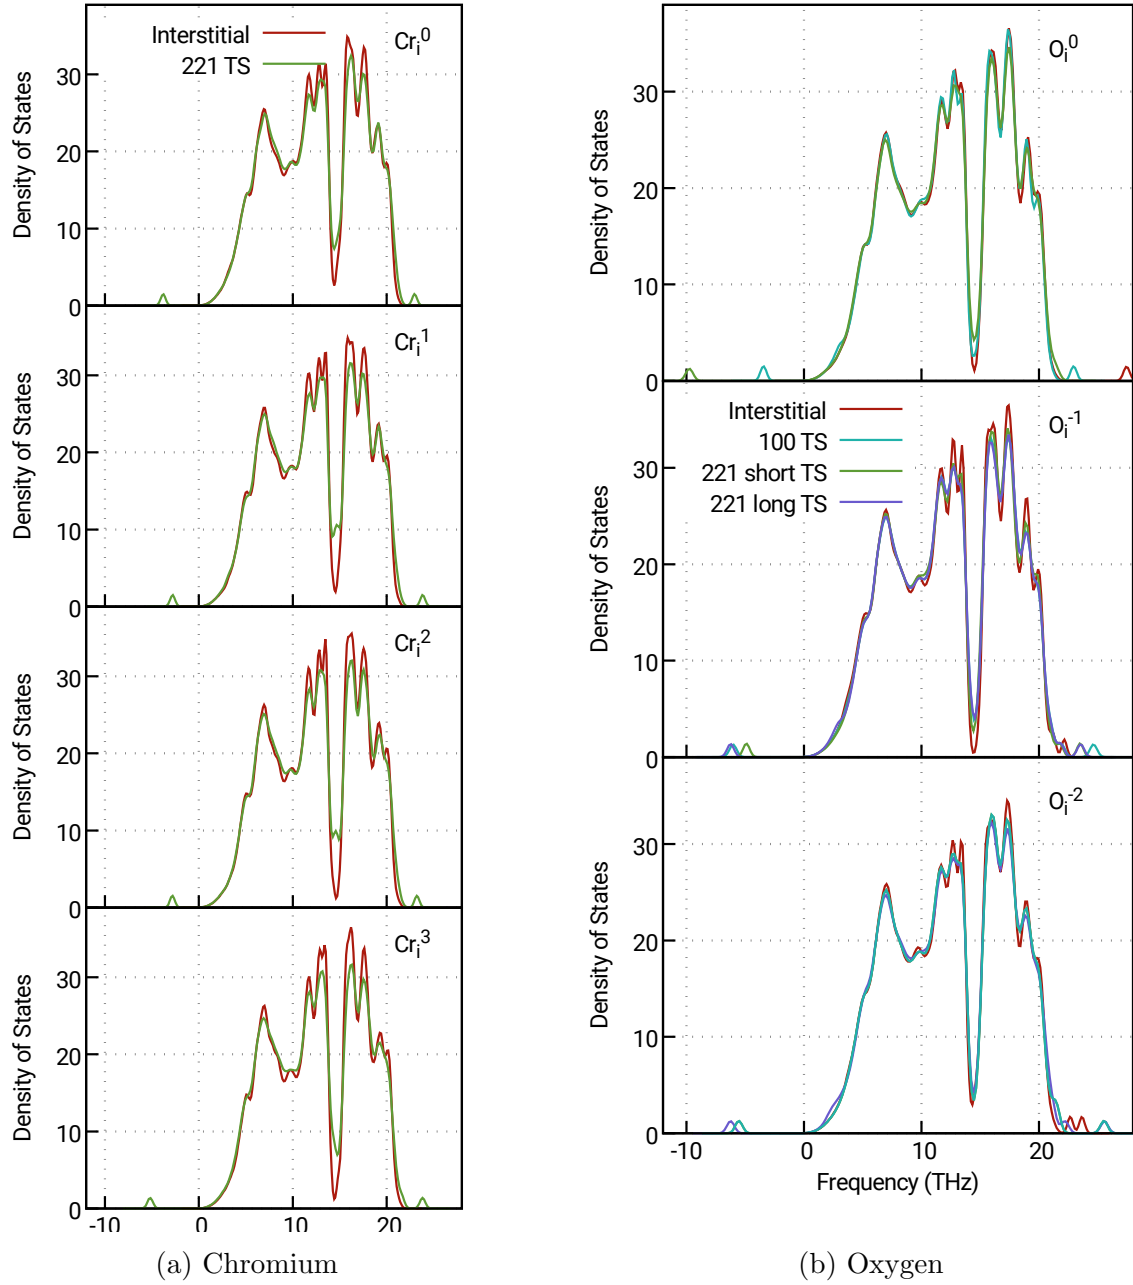

Figure S3: Phonon density of states of the interstitials and the transition states for (a) Cr interstitial diffusion and (b) O interstitial diffusion. Imaginary frequencies are plotted as negative frequencies. The pathways for Cr and O interstitial diffusion are described in Fig. 8 in the main article. In the case of  $\text{O}_i^{-2}$ , phonon DOS for the transition states corresponding to [221]-short and [100] pathways are identical.

# Preliminary Data for Finite Temperatures

Concentration of a defect is a function of its formation energy,  $E_f$ ,

$$c = c_0 e^{-\beta E_f}, \quad (1)$$

with  $c_0$  being lattice site number.

The effect of pressure and temperature is accounted for through the chemical potential term in the defect formation energetics. We utilized grand canonical formalism to compute the elemental chemical potentials at finite temperatures. In this formalism, bulk  $\text{Cr}_2\text{O}_3$  is supposed to be in contact with  $\text{O}_2$  reservoir at temperature,  $T$ , and partial pressure,  $p_{\text{O}_2}$ . The oxygen chemical potential is defined as

$$\mu_{\text{O}}(p_{\text{O}_2}, T) = \mu_{\text{O}}^0 + \Delta\mu_{\text{O}}^0(1\text{atm}, 298\text{K}) + \Delta\mu_{\text{O}}(p_{\text{O}_2}, T). \quad (2)$$

In the above equation,  $\mu_{\text{O}}^0$  is the 0 K DFT computed O chemical potential,  $\Delta\mu_{\text{O}}^0(1\text{atm}, 298\text{K})$  is the correction to obtain the experimental chemical potential of O at standard conditions, and  $\Delta\mu_{\text{O}}(p_{\text{O}_2}, T)$  is given as

$$\Delta\mu_{\text{O}}(p_{\text{O}_2}, T) = kT \ln(p_{\text{O}_2}), \quad (3)$$

and obtained from NIST-JANAF tables. Cr chemical potential,  $\mu_{\text{Cr}}$ , is obtained from  $\mu_{\text{O}}$  as

$$\mu_{\text{Cr}}(p_{\text{O}_2}, T) = \Delta H_{\text{Cr}_2\text{O}_3} - \mu_{\text{O}}(p_{\text{O}_2}, T), \quad (4)$$

where  $\Delta H_{\text{Cr}_2\text{O}_3}$  is the formation enthalpy of  $\text{Cr}_2\text{O}_3$ . Recalling the formation energy of a charged defect as

$$E_f^{X_s^q} = E_{\text{tot}}^{X_s^q} - E_{\text{tot}}^{\text{bulk}} + \sum_{s'} n_{s'}(X_s^q) \mu_{s'} + qE_F + E_{\text{corr}}^{X_s^q}, \quad (5)$$

it is clear that defect concentrations are a function of temperature, pressure, and Fermi level.

$$c^{X_s^q} \equiv c^{X_s^q}(p_{O_2}, T, E_F). \quad (6)$$

Since the overall system is charge neutral, defect concentrations are constrained by charge neutrality condition, which is defined as

$$\sum_{X_s^q} q c^{X_s^q} + p - n = 0, \quad (7)$$

where  $p$  and  $n$  represent the number of holes and electrons respectively. The number of free electrons,  $n$ , is given by

$$n(T, E_F) = \int_{CBM}^{\infty} f_{FD}(E, T, E_F) g(E) dE, \quad (8)$$

where  $g(E)$  is the density of states, and  $f_{FD}$  is the Fermi-Dirac distribution function defined as

$$f_{FD}(E, T, E_F) = \frac{1}{1 + e^{(E-E_F)/kT}}. \quad (9)$$

Similarly the number of free holes,  $p$ , is given by

$$p(T, E_F) = \int_{-\infty}^{VBM} (1 - f_{FD}(E, T, E_F)) g(E) dE. \quad (10)$$

Substituting the definitions of defect concentrations, electron and hole numbers in Eqn. 7, and by making  $T$  and  $p_{O_2}$  as free variables, we can solve for  $E_F$  in terms of  $T$  and  $p_{O_2}$ . Since,  $E_F$  is a function of  $T$  and  $p_{O_2}$ ,  $E_F$  can be eliminated from Eq. 6 and Eq. 6 is rewritten as

$$c^{X_s^q} \equiv c^{X_s^q}(p_{O_2}, T). \quad (11)$$

From the evaluated defect concentrations, one could compute composition deviations as a



function of  $T$  and  $p_{O_2}$  trivially. In figures S4 and S5, interstitials investigated in the main article and the vacancies investigated in Ref. [ 13] are accounted for.

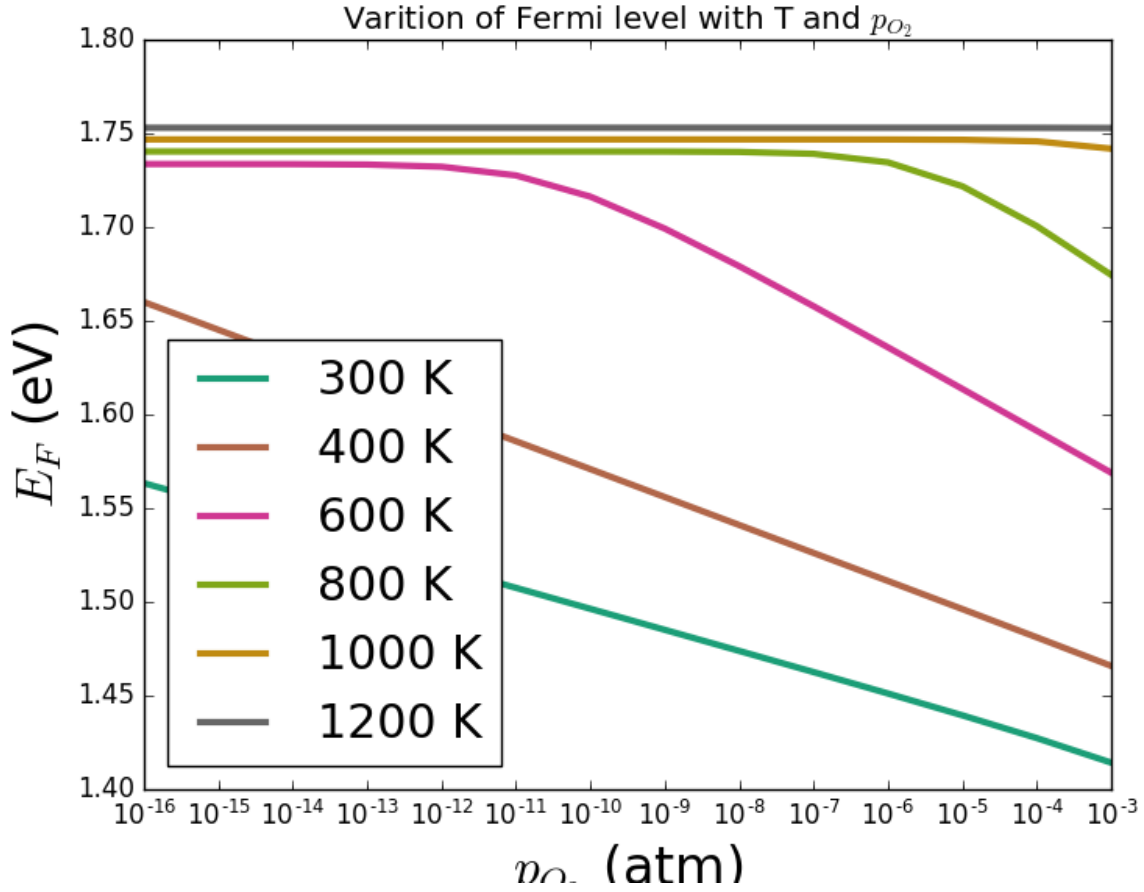

Figure S4: Fermi level as a function of temperature and oxygen partial pressure in undoped  $\text{Cr}_2\text{O}_3$ .

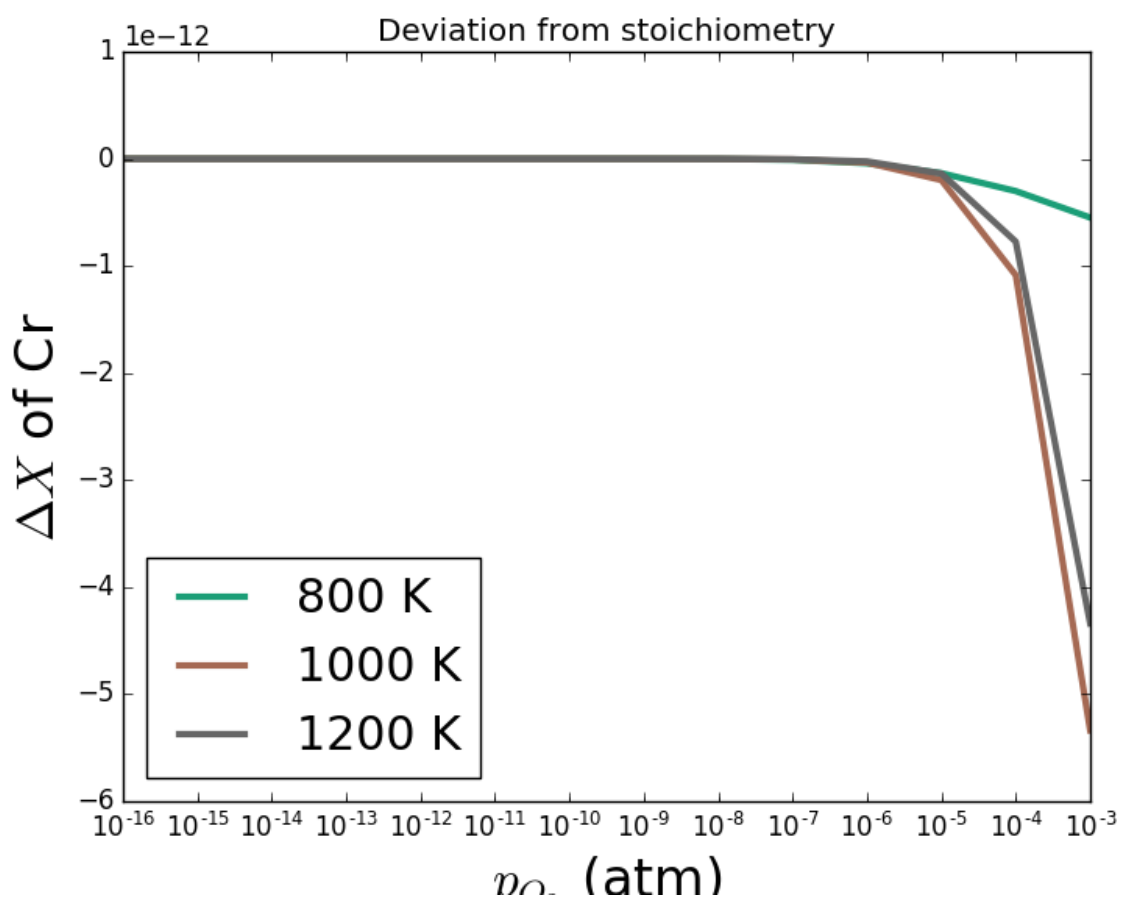

Figure S5: Deviation of Cr composition from stoichiometry in  $\text{Cr}_2\text{O}_3$  as a function of temperature and oxygen partial pressure.

# Electronic structure of Transition States

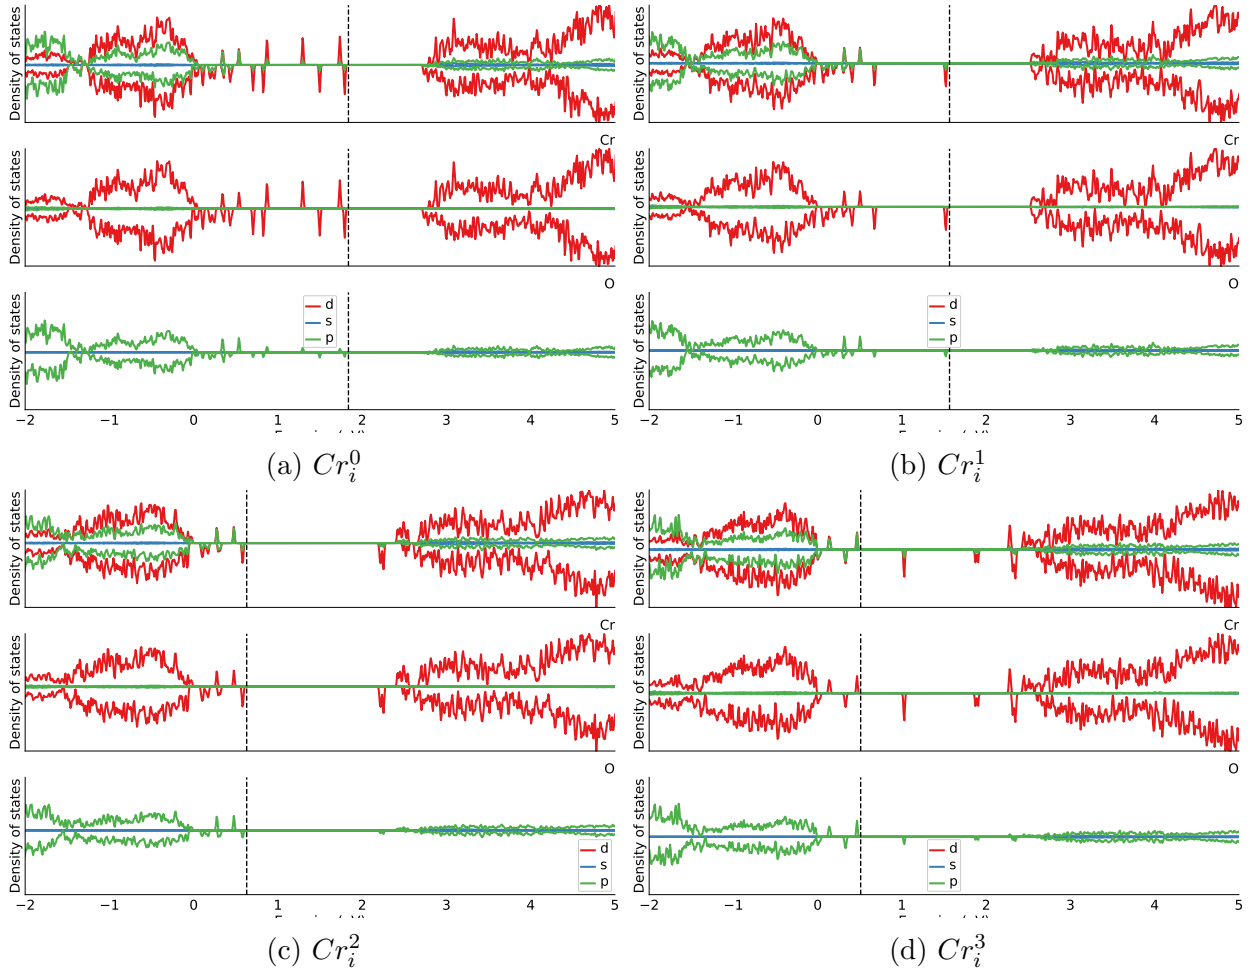

Figure S6: Electronic density of states (DOS) at the transition states of the  $Cr_i$  for (a) 0, (b) 1, (c) 2, and (d) 3 charge states along the [221] path way. The 0-level of the x-axis is at the average Hartree potential.

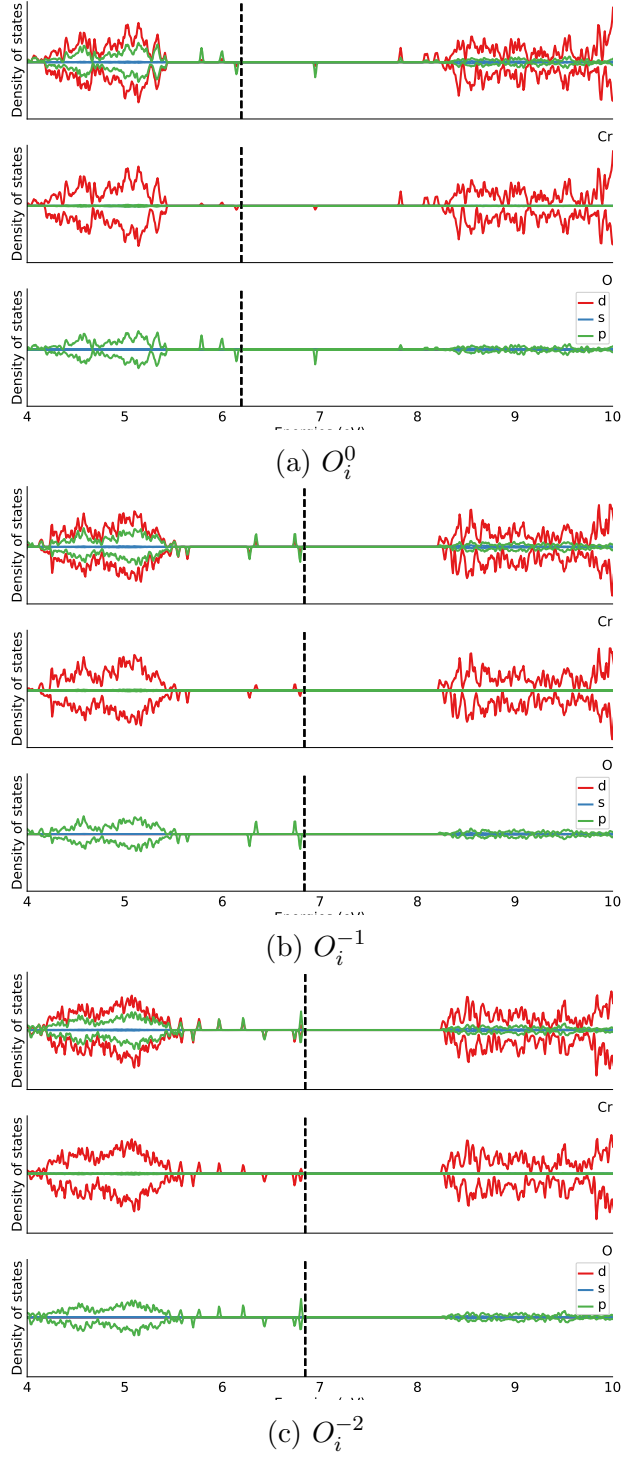

Figure S7: Electronic density of states (DOS) at the transition states of the  $O_i$  for (a) 0, (b) -1, and (c) -2 charge states along the  $[100]$  path way. The 0-level of the x-axis is at the average Hartree potential.

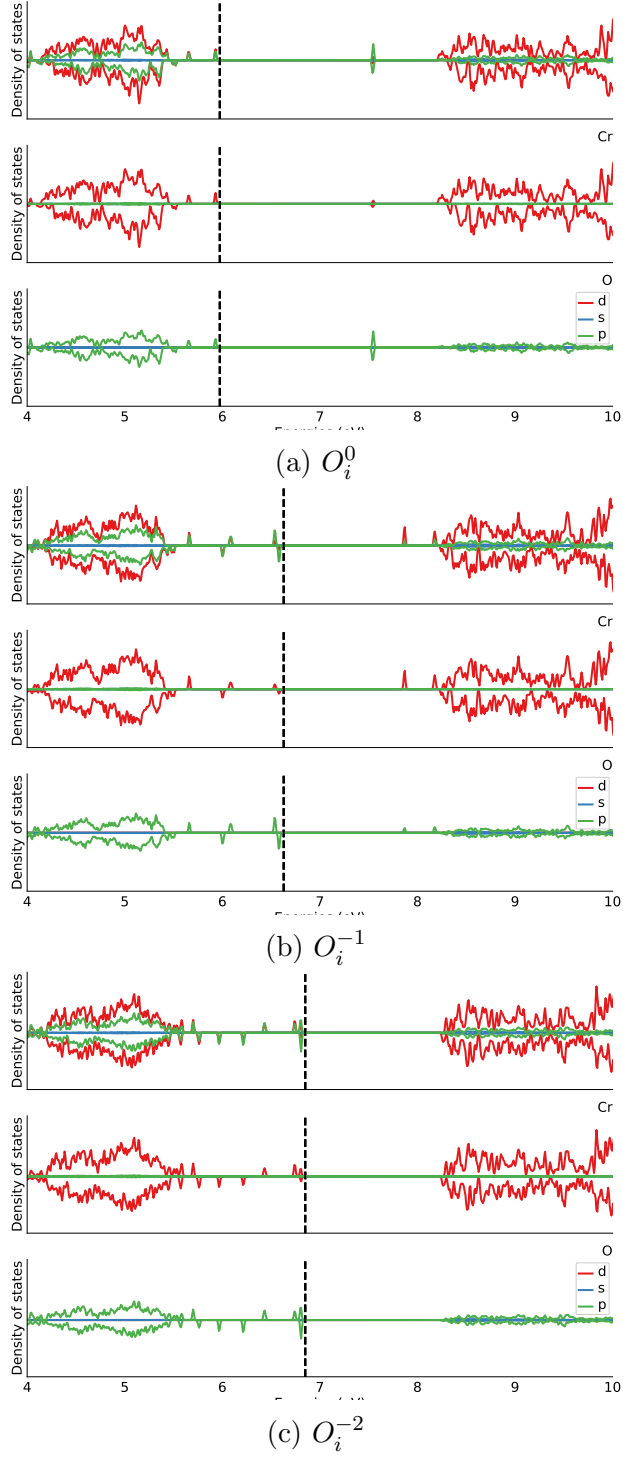

Figure S8: Electronic density of states (DOS) at the transition states of the  $O_i$  for (a) 0, (b) -1, and (c) -2 charge states along the [221]-short path way described in the main article. The 0-level of the x-axis is at the average Hartree potential.

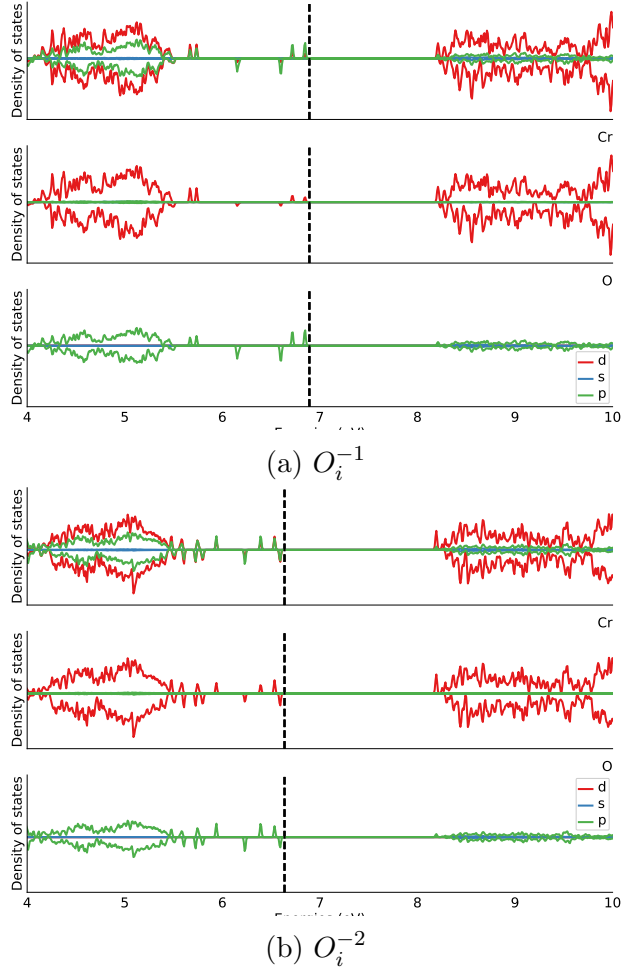

Figure S9: Electronic density of states (DOS) at the transition states of the  $O_i$  for (a) -1, and (b) -2 charge states along the [221]-long path way described in the main article. The 0-level of the x-axis is at the average Hartree potential of the supercell.

# Local Electrostatic Potential Experienced by Diffusing Ion

Table S6: Local electrostatic potential (LEP) experienced by the diffusing Cr/O ion in various charge states at the transition states (TS) of the pathways considered in the main article. The values are given with respect to the LEP at the corresponding interstitial ground states.

| Defect | q  | $\Delta\text{LEP at TS (V)}$ |             |            |
|--------|----|------------------------------|-------------|------------|
|        |    | [100]                        | [221] short | [221] long |
| $O_i$  | 0  | 1.71                         | 0.39        | —          |
|        | -1 | 0.50                         | 0.42        | 0.80       |
|        | -2 | 0.49                         | 0.49        | -0.39      |
| $Cr_i$ |    | [100]                        | [221]       |            |
|        | 0  | 1.42                         | -0.54       |            |
|        | 1  | 1.23                         | 1.33        |            |
|        | 2  | 1.77                         | 2.35        |            |
|        | 3  | -0.31                        | 0.51        |            |

## References

- (1) Kresse, G.; Hafner, J. *Phys. Rev. B* **1993**, *47*, 558–561.
- (2) Kresse, G.; Hafner, J. *Phys. Rev. B* **1994**, *49*, 14251–14269.
- (3) Kresse, G.; Furthmüller, J. *Phys. Rev. B* **1996**, *54*, 11169–11186.
- (4) Perdew, J. P.; Ruzsinszky, A.; Csonka, G. I.; Vydrov, O. A.; Scuseria, G. E.; Constantin, L. A.; Zhou, X.; Burke, K. *Phys. Rev. Lett.* **2008**, *100*, 136406.
- (5) Blöchl, P. E. *Phys. Rev. B* **1994**, *50*, 17953–17979.
- (6) Kresse, G.; Joubert, D. *Phys. Rev. B* **1999**, *59*, 1758–1775.
- (7) Dudarev, S. L.; Botton, G. A.; Savrasov, S. Y.; Humphreys, C. J.; Sutton, A. P. *Phys. Rev. B* **1998**, *57*, 1505–1509.

- (8) Kumagai, Y.; Oba, F. *Phys. Rev. B* **2014**, *89*, 195205.
- (9) Freysoldt, C.; Neugebauer, J.; Van de Walle, C. G. *Phys. Rev. Lett.* **2009**, *102*, 016402.
- (10) Broberg, D.; Medasani, B.; Zimmermann, N. E.; Yu, G.; Canning, A.; Haranczyk, M.; Asta, M.; Hautier, G. *Computer Physics Communications* **2018**, *226*, 165 – 179.
- (11) Janotti, A.; Van de Walle, C. G. *Phys. Rev. B* **2007**, *76*, 165202.
- (12) Togo, A.; Tanaka, I. *Scr. Mater.* **2015**, *108*, 1–5.
- (13) Medasani, B.; Sushko, M. L.; Rosso, K. M.; Schreiber, D. K.; Bruemmer, S. M. *The Journal of Physical Chemistry C* **2017**, *121*, 1817–1831.
